# Supplementary material for: Unsupervised learning of quantum many-body scars using intrinsic dimension
Source: arXiv:2401.07795 source file (2024-02-01)
Supplement: Supplementary file 1 [file appendix.tex]

\title{Appendix}

In order to appreciate why the PEM metric between time-evolved quantum states gives us the ability to distinguish between scar and thermal phases, we observe that this measure is predominantly dependent on two quantities: the projection of the state on the computational basis and the expansion coefficients in the energy eigenbasis. For thermal initial states, there is minimal overlap with computational basis states and hence also the product states with which we quench the system from. Furthermore, the energy expansion coeffients are shown to be lower 
Furthermore, the energy expansion coefficients are shown to be distributed in a Gaussian distribution [ref], which leads to dephasing over terms in the distance measure leading to the initial stat

For quenching from scar initial states, 

The conventional approach has been "manual"

analagous to the standard "manual" approach for detecting quantum single-body scars (meta-learning paper)

1. Show that the decay rate for time evolved states using the HS metric is faster than the periodicity of the scar states, so cannot distinguish. For the EM distance, because it is dependent on the overlap with product state computational basis, the decay rate is slower for scar states which is why it is possible to distinguish between the two phases.

2. Plots for distribution of probability amplitudes for two cases

3. Plots for HS and TEM 

4. Write about the MDS optimisation in terms of strings and forces - for scars, there is an attractive force which pulls embedded points together. For thermal states, there is no force so the points are scattered uniformly.

The earth mover's distance makes use of the reviving overlap with the product states (by using measures in computational basis) to amplify the lack of dephasing in scar phase.

Additions:

Need to stress the experimental advantage of our method over typical methods for studying quantum scars (e.g. picking a local observable and measuring)

we're somewhere between tomography and single observable because we pick a basis to measure in
